# Supplementary material for: Unselfie: Translating Selfies to Neutral-pose Portraits in the Wild
Source: arXiv:2007.15068 source file (2020-07-29)
Supplement: Supplementary file 1 [file supp_Fig_inpaintBG.tex]

\begin{figure}
\centering
% \captionsetup{justification=centering}
\captionsetup{font=small,labelfont=normalsize,justification=centering}

\begin{subfigure}[b]{.19\linewidth}
\caption*{Input selfie}
\vspace{-1mm}
\begin{overpic}[width=\linewidth]{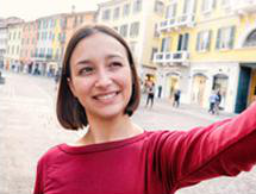}
\put(0,665) {\scalebox{0.65}{\id{206713499}}}
\end{overpic}
\end{subfigure}
\begin{subfigure}[b]{.19\linewidth}
% \caption*{Input BG $I_{bg}$}
\caption*{BG $I_{bg}$}
\vspace{-1mm}
\includegraphics[width=\linewidth]{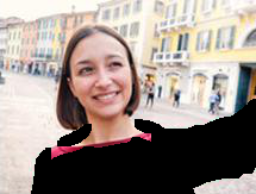}
\end{subfigure}
\begin{subfigure}[b]{.19\linewidth}
% \caption*{Input inpainted BG $I_{bg}$}
\caption*{Inpainted BG $I_{ibg}$}
\vspace{0mm}
\includegraphics[width=\linewidth]{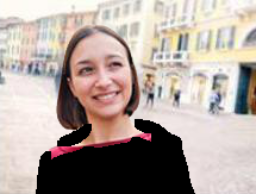}
\end{subfigure}
\begin{subfigure}[b]{.19\linewidth}
% \caption*{Result}
\caption*{Result with $I_{bg}$}
\vspace{-1mm}
\includegraphics[width=\linewidth]{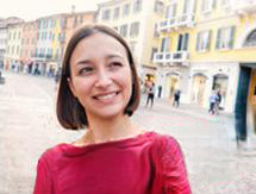}
\end{subfigure}
\begin{subfigure}[b]{.19\linewidth}
% \caption*{Result \\(inpainted BG)}
\caption*{Result with $I_{ibg}$}
\vspace{0mm}
\includegraphics[width=\linewidth]{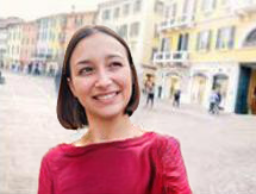}
\end{subfigure}

\begin{subfigure}[b]{.19\linewidth}
% \caption*{Input selfie}
\vspace{-1mm}
\begin{overpic}[width=\linewidth]{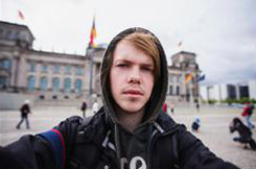}
\put(0,665) {\scalebox{0.65}{\id{138378456}}}
\end{overpic}
\end{subfigure}
\begin{subfigure}[b]{.19\linewidth}
% \caption*{Ours}
\vspace{-1mm}
\includegraphics[width=\linewidth]{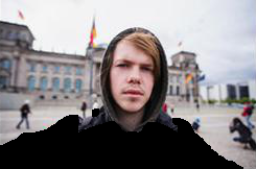}
\end{subfigure}
\begin{subfigure}[b]{.19\linewidth}
% \caption*{Ours \\(inpainted background)}
\vspace{0mm}
\includegraphics[width=\linewidth]{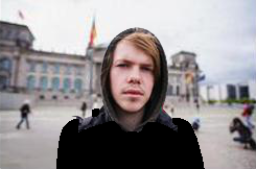}
\end{subfigure}
\begin{subfigure}[b]{.19\linewidth}
% \caption*{Ours}
\vspace{-1mm}
\includegraphics[width=\linewidth]{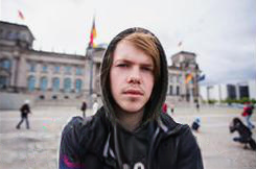}
\end{subfigure}
\begin{subfigure}[b]{.19\linewidth}
% \caption*{Ours \\(inpainted background)}
\vspace{0mm}
\includegraphics[width=\linewidth]{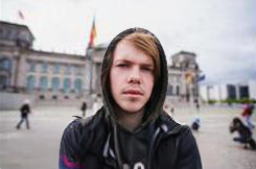}
\end{subfigure}

\begin{subfigure}[b]{.19\linewidth}
% \caption*{Input selfie}
\vspace{-1mm}
\begin{overpic}[width=\linewidth]{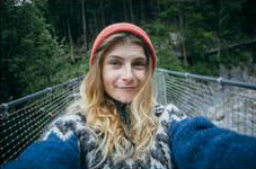}
\put(0,665) {\scalebox{0.65}{\id{225137362}}}
\end{overpic}
\end{subfigure}
\begin{subfigure}[b]{.19\linewidth}
% \caption*{Ours}
\vspace{-1mm}
\includegraphics[width=\linewidth]{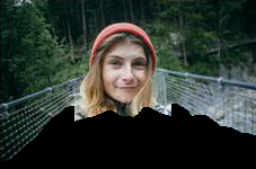}
\end{subfigure}
\begin{subfigure}[b]{.19\linewidth}
% \caption*{Ours \\(inpainted background)}
\vspace{0mm}
\includegraphics[width=\linewidth]{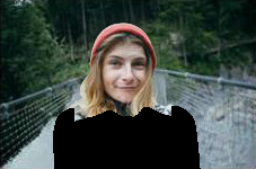}
\end{subfigure}
\begin{subfigure}[b]{.19\linewidth}
% \caption*{Ours}
\vspace{-1mm}
\includegraphics[width=\linewidth]{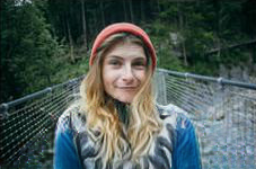}
\end{subfigure}
\begin{subfigure}[b]{.19\linewidth}
% \caption*{Ours \\(inpainted background)}
\vspace{0mm}
\includegraphics[width=\linewidth]{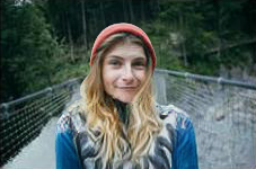}
\end{subfigure}

\caption{Results of using inpaited background.}
\label{supp_fig:inpaintBG}
\end{figure}
